# Supplementary material for: Geometry of Rounding: Near Optimal Bounds and a New Neighborhood Sperner's Lemma
Source: arXiv:2304.04837 source file (2023-04-10)
Supplement: Supplementary file 1 [file appendix_asymptotics.tex]

\section{Asymptotics}

\begin{fact}\label{x-plus-one-to-the-one-over-x}
The following limit holds:
\[
\lim_{x\to\infty}(x+1)^\frac{1}{x} = 1
\]
\end{fact}
% \begin{proof}
% This is a standard fact that is typically proved with L'Hopital's rule, but we offer a fun proof using the AM-GM inequality. 
% \end{proof}
% \todo[inline]{Include a proof}

\begin{proposition}[Subexponential Functions]\label{subexponential-equivalence}
The following function classes are equivalent:
\[
2^{o(n)} = \bigcap_{c\in(1,\infty)} o(c^n) = \bigcap_{c\in(1,\infty)} O(c^n)
\]
\end{proposition}
\begin{proof}

% \todo[inline]{Check nuances of the definition of little-o being equivalent to the limit definition}
We first show the second equality. For any constant $c\in(1,\infty)$, we have $o(c^n) \subseteq O(c^n) \subseteq o((2c)^n)$, and since the intersections are over all constants including $c'=2c$, the equality holds\footnote{To see that $O(c^n) \subseteq o((2c)^n)$, consider $f\in O(c^n)$. Thus, $\lim_{n\to\infty}\frac{f(n)}{c^n}$ is equal to some constant $C$, and thus we can show that $f\in o((2c)^n)$ by showing that $\lim_{n\to\infty}\frac{f(n)}{(2c)^n}=0$ which is true because $\lim_{n\to\infty}\frac{f(n)}{(2c)^n}=\left[\lim_{n\to\infty}\frac{f(n)}{c^n}\right]\cdot\left[\lim_{n\to\infty}\frac{c^n}{(2c)^n}\right]=C\cdot0=0$.}.

We now prove the superset $(\supseteq)$ containment of the first equality. Let $f\in\bigcap_{c\in(1,\infty)} o(c^n)$. To show that $f\in2^{o(n)}$ we must show (by definition) that $\lg2\circ f\in o(n)$. That is, (by definition) we must show that for any $\varepsilon\in(0,\infty)$ there exists $N_\varepsilon$ such that for all $n\geq N_\varepsilon$ it holds that $\lg2(f(n))\leq\varepsilon n$. So let $\varepsilon\in(0,\infty)$ be arbitrary. Let $\delta=1$ and $c=2^\varepsilon$ noting that $c>1$ because $\varepsilon>0$, so $f\in o(c^n)$. Then, by definition, there exists some $N_\delta$ such that for all $n\geq N_\delta$ it holds that $f(n)\leq\delta c^n$. Let $N_\varepsilon=N_\delta$. This implies for all $n\geq N_\varepsilon=N_\delta$ that
\begin{align*}
\lg2(f(n)) &\leq \lg2(\delta c^n) \\
&= \lg2(c^n) \tag{$\delta=1$} \\
&= \lg2((2^\varepsilon)^n) \tag{$c=2^\varepsilon$} \\
&= \varepsilon n
\end{align*}
This shows that $f\in 2^{o(n)}$.

Lastly, we prove the subset ($\subseteq$) containment of the first equality. Let $f\in 2^{o(n)}$ be arbitrary. To show that $f\in \bigcap_{c\in(1,\infty)} o(c^n)$, let $c\in(1,\infty)$ be arbitrary and we will show that $f\in o(c^n)$ by the definition. Let $\varepsilon\in(0,\infty)$ be arbitrary, and let $\delta=\frac{\lg2(c)}{2}$ (noting that since $c>1$, $\delta>0$. Since $f\in 2^{o(n)}$, we have $\lg2\circ f\in o(n)$, so by definition there exists some $N_\delta$ such that for all $n\geq N_\delta$ it holds that $\lg2(f(n))\leq\delta n$. Let $N_\varepsilon=\max(N_\delta,\ceil{\frac{-2\lg2(\varepsilon)}{\lg2(c)}})$. We have that for all $n\geq N_\varepsilon$ that
\begin{align*}
    \lg2(f(n)) &\leq \delta n \tag{$n\geq N_\varepsilon \geq N_\delta$} \\
               &= \frac{n\lg2(c)}{2} \\
               &\leq \lg2(\varepsilon) + n\lg2(c) \tag{$n\geq N_\varepsilon \geq \ceil{\frac{-2\lg2(\varepsilon)}{\lg2(c)}}$} \\
               &= \lg2(\varepsilon c^n)
\end{align*}
By monotonicity of $\lg2$, this implies for $n\geq N_\varepsilon$ that $f(n)\leq \varepsilon c^n$. Since $\varepsilon$ was arbitrary, this shows $f\in o(c^n)$, and since $c$ was also arbitrary, this shows $f\in \bigcap_{c\in(1,\infty)} o(c^n)$.
\end{proof}

\begin{fact}\label{powers-of-sub-one-convergence}
If $f:\N\to\R$ has $\lim_{n\to\infty}f(n)=\ell$ for some $\ell\in(-1,1)$, then $\lim_{n\to\infty}f(n)^n=0$.
\end{fact}
\begin{proof}
We show this by the definition of limit, so let $\varepsilon\in(0,\infty)$ be arbitrary. Pick some $\gamma\in(\abs{\ell},1)$ noting that $\ell\in(-\gamma, \gamma)\subsetneq (-1,1)$. Since $\gamma\in(0,1)$, $\lim_{n\to\infty}\gamma^n=0$, so let $N_1$ be such that for $n\geq N_1$ it holds that $\gamma^n<\varepsilon$. And since $f(n)$ converges to $\ell\in(-\gamma,\gamma)$, let $N_2$ be such that for $n\geq N_2$ we have $\abs{f(n)}<\gamma$. Thus, for $n\geq N\defeq\max\set{N_1,N_2}$ we have
\[
\abs{f(n)^n} = \abs{f(n)}^n \leq \gamma^n < \varepsilon
\]
so $\lim_{n\to\infty}f(n)^n=0$.
\end{proof}

\begin{lemma}\label{one-convergence-powers-sub-exponential}
If $g:\N\to[0,\infty)$ is such that $\lim_{n\to\infty}g(n)=1$, then for $h:\N\to\R$ defined by $h(n) = g(n)^n$ we have $h\in 2^{o(n)}$.
\end{lemma}
\begin{proof}
Using \Autoref{subexponential-equivalence}, we will show for all $c\in(1,\infty)$ that $h\in o(c^n)$. Let $c\in(1,\infty)$ be arbitrary for this purpose. Then
\[
\frac{h(n)}{c^n} = \left(\frac{g(n)}{c}\right)^n
\]
and since $g(n)$ converges to $1$ and $c>1$, $\frac{g(n)}{c}$ converges to $\frac1c\in(0,1)$, so by \Autoref{powers-of-sub-one-convergence}, $\left(\frac{g(n)}{c}\right)^n$ converges to $0$. Thus $\lim_{n\to\infty}\frac{h(n)}{c^n}=0$, so $h\in o(c^n)$.

\end{proof}

\begin{lemma}[Asymptotic Logs]\label{asymptotic-logs-lemma}
If $f,g:\N\to(0,\infty)$ such that $\ln(f(n))\in o(\ln(g(n))$ and either $\lim_{n\to\infty}g(n)=\infty$ or $\lim_{n\to\infty}g(n)<1$, then $f(n)\in o(g(n))$.
\end{lemma}
\begin{proof}
For any $C\in(0,\infty)$, there exists $N_C\in\N$ such that for $n\geq N_C$ we have $\ln(f(n)) \leq C\ln(g(n))=(\ln(g(n)^C))$, so exponentiating, we have for $n\geq N_C$ that $f(n) \leq g(n)^C$.

For the first case, if $\lim_{n\to\infty}g(n)=\infty$ then take $C=\frac12$ above. Let $\delta\in(0,\infty)$ be arbitrary, and let $N_\delta\in\N$ be such that for $n\geq N_\delta$, $g(n)\geq\frac{1}{\delta^2}$. Let $N=\max(N_C, N_\delta)$. Then for $n\geq N$ we have
\begin{align*}
    f(n) &\leq g(n)^{\frac12} &= \frac{1}{\sqrt{g(n)}}\cdot g(n) \tag{$C=\frac12$ and $n\geq C$} \\
    &\leq \frac{\sqrt{\frac{1}{\delta^2}}} g(n) = \delta g(n) \tag{$n\geq N_\delta$}
\end{align*}
which shows $f(n)\in o(g(n))$.

For the second case, if $\lim_{n\to\infty}g(n)<1$, then let $\ell$ denote this limit. Let $\delta\in(0,\infty)$ be arbitrary. Take $C$ to be such that $\ell^{\frac{C-1}{2}}<\delta$. Since $\ell\in(0,1)$, $\sqrt(\ell)>\ell$. Let $N_\delta\in\N$ be such that for $n\geq N_\delta$, $g(n)\leq\sqrt(\ell)$. Let $N=\max(N_C, N_\delta)$. Then for $n\geq N$ we have
\begin{align*}
    f(n) &\leq g(n)^C &= g(n)^{C-1}\cdot g(n) \tag{$n\geq N_C$}\\
    & \leq {\sqrt{\ell}}^{C-1}\cdot g(n) \tag{$n\geq N_\delta$ and a positive power is an increasing function} \\
    &\leq \delta g(n) \tag{Choice of $C$}
\end{align*}
which shows $f(n)\in o(g(n))$.

\end{proof}

\begin{remark}
If the two limit conditions on $g$ above are removed, the conclusion may not hold. For example, let $C_f\in(0,1)$ and $C_g\in[1,\infty)$ and suppose that $f,g:\N\to(0,\infty)$ are such that $\lim_{n\to\infty}f(n)=C_f$ and $\lim_{n\to\infty}g(n)=C_g$. Then by continuity, $\lim_{n\to\infty}\ln(f(n))=\ln(C_f)<0$ (since $C_f<1$) and for any $\delta\in(0,\infty)$, $\lim_{n\to\infty}\delta \ln(g(n)) = \delta \ln(C_g)\geq0$ (since $C_g\geq1$). Thus, for sufficiently large $n\in\N$, $\ln(f(n)) \leq \delta \ln(g(n))$ showing that $\ln(f(n))\in o(\ln(g(n))$. However, as both $f$ and $g$ have finite limits, $f(n)\in \Theta_n(1)$ and $g(n)\in \Theta_n(1)$ so $f(n)\not\in o(g(n))$.
\end{remark}
