# Supplementary material for: Geometry of Rounding: Near Optimal Bounds and a New Neighborhood Sperner's Lemma
Source: arXiv:2304.04837 source file (2023-04-10)
Supplement: Supplementary file 2 [file appendix_asymptotics_not_used.tex]

\begin{lemma}
If $f\in\omega(\frac{\ln(n)}{n})$ then $(1+f(n))^n\not\in\bigcup_{k\in\N}O(n^k)$. That is, $(1+f(n))^n$ is asymptotically larger than every polynomial.
\end{lemma}
\begin{proof}
For each $k\in\N$, we show that $n^k\in o((1+f(n))^n)$. By \Autoref{asymptotic-logs-lemma}, since $\lim_{n\to\infty}(1+f(n))^n=\infty$ (see footnote\footnote{For any any $r\in\R$, $\lim_{n\to\infty}(1+\frac{r}{n})^n=e^r$ is a standard fact, so for any $r\in\R$, $\lim_{n\to\infty}(1+\frac{\ln(n)}{n})^n\geq e^r$ which shows that the limit is $\infty$, and thus $\lim_{n\to\infty}(1+f(n))^n=\infty$ as well since $f(n)\in\omega(\frac{\ln(n)}{n})$}), it suffices to consider the logarithms and show that $\ln(n^k)\in o(\ln((1+f(n))^n))$. To show this, observe the following limit\footnote{Morally, $\left(1+C\frac{\ln(n)}{n}\right)^n$ is asymptotically like $e^{C\ln(n)}=n^C$ and so asymptotically the ratio of the logarithm of $\left(1+C\frac{\ln(n)}{n}\right)^n$ to the logarithm of $n^k$ is $\frac{\ln(n^C)}{\ln(n^k)}=\frac{C\ln(n)}{k\ln(n)}=\frac{C}{k}$.} for any $C\in(0,\infty)$.
\begin{align*}
    \lim_{n\to\infty}\frac{\ln\left(\left(1+C\frac{\ln(n)}{n}\right)^n\right)}{\ln(n^k)} &=     \lim_{n\to\infty}\frac{n\ln\left(1+C\frac{\ln(n)}{n}\right)}{k\ln(n)} \tag{Logarithm properties}\\
    &= \lim_{n\to\infty}\frac{\ln\left(1+C\frac{\ln(n)}{n}\right)\quad\to0}{k\frac{\ln(n)}{n}\quad\to0} \tag{Divide numerator and denominator by $n$}\\
    &= \lim_{n\to\infty}\frac{\left( \frac{1}{1+C\frac{\ln(n)}{n}}\right)\cdot C\cdot \frac{d}{dn}\left[\frac{\ln(n)}{n}\right] }{k\cdot\frac{d}{dn}\left[\frac{\ln(n)}{n}\right]} \tag{L'Hopital's rule}\\
    &= \lim_{n\to\infty}\frac{\left( \frac{1}{1+C\frac{\ln(n)}{n}}\right)\cdot C}{k} \tag{Simplify}\\
    &= \frac{C}{k} \tag{Evaluate}
\end{align*}
Thus, for any $C\in\R$ we have 
\[
    \lim_{n\to\infty}\frac{\ln\left((1+f(n))^n\right)}{\ln(n^k)} \geq     \lim_{n\to\infty}\frac{\ln\left((1+C\frac{\ln(n)}{n})^n\right)}{\ln(n^k)} = \frac{C}{k}
\]
and since this holds for arbitrarily large $C$, we conclude that
\[
  \lim_{n\to\infty}\frac{\left((1+f(n))^n\right)}{\ln(n^k)} = \infty.
\]
\end{proof}
