# Supplementary material for: Geometry of Rounding: Near Optimal Bounds and a New Neighborhood Sperner's Lemma
Source: arXiv:2304.04837 source file (2023-04-10)
Supplement: Supplementary file 3 [file appendix_other_not_used.tex]

\begin{lemma}
For any $d\in\N$, if $n\in[d]$, then $\ceil{n\cdot\frac{d+1}{d}}=n+1$.
\end{lemma}
\begin{proof}
We have that $n\cdot\frac{d+1}{d}>n$, and since $n$ is an integer that means $\ceil{n\cdot\frac{d+1}{d}}>n$. Also, since $n\leq d$ we get the following equivalent statements:
\begin{align*}
    n\leq d &\iff nd+n \leq nd+d \tag{Add $nd$ to both sides}\\
    &\iff n(d+1) \leq d(n+1) \tag{Factor both sides} \\
    &\iff n\cdot\frac{d+1}{d} \leq n+1 \tag{Divide both side by $d>0$} \\
    &\iff \ceil{n\cdot\frac{d+1}{d}} \leq \ceil{n+1}=n+1 \tag{Ceiling of both sides} \\
\end{align*}
Thus, we have $n<\ceil{n\cdot\frac{d+1}{d}}\leq n+1$, and so we get equality with $n+1$.
\end{proof}

\todo[inline]{When showing that the iterated ceiling is greater than or equal to $d+1$, I can use this result on the value of $\epsilon=\frac{1}{2d}$ to show that it is exactly equal to $d+1$, or I can argue that it is a strictly increasing sequence with $d$ terms and the first term is $\geq2$}

\begin{porism}
For any $d\in\N$, if $n\in[d]$, then for any $\epsilon\in(0,\frac{d+1}{d}]$, $\ceil{n\cdot\epsilon}=n+1$.
\end{porism}
\begin{proof}
The same proof above can be used noting that in the last step we have $n<\ceil{n\cdot\epsilon}\leq\ceil{n\cdot\frac{d+1}{d}}\leq n+1$.
\end{proof}
